# Supplementary material for: Semi-Supervised Text Classification via Self-Pretraining
Source: arXiv:2109.15300 source file (2021-09-30)
Supplement: Supplementary file 1 [file doc-appendix.tex]

% %%
% %% If your work has an appendix, this is the place to put it.
% \appendix
% \section{Research Methods}
% \subsection{Part One}
% BLANK BLANK BLANK BLANK BLANK 
% \subsection{Part Two}
% BLANK BLANK BLANK BLANK BLANK 
% \section{Online Resources}
% BLANK BLANK BLANK BLANK BLANK 
